# Supplementary material for: Stochastic Interpolants via Conditional Dependent Coupling
Source: arXiv:2509.23122 source file (2026-10-29)
Supplement: Supplementary file 1 [file proof_2.tex]

\subsection{Proof of Theorem~\ref{theorem:lowerTrainingTime}} \label{pf:fasterTrain}
We provide a formal proof demonstrating that an efficiently designed Flow Matching model with conditional dependent coupling achieves a lower training time than a direct, single-stage model for high-resolution image generation, as stated in Theorem~\ref{theorem:lowerTrainingTime}.

\begin{proof}
Let
\[
\tau_A \;\triangleq\; \tau\!\big(x_0 \to \hat{x}_1\big), \qquad
\tau_k \;\triangleq\; \tau\!\big(x_0^{(k)} \to \hat{x}_1^{(k)}\big), \; 1\le k\le K,
\]
so that $T_A=\mathbb{E}[\tau_A]$ and, under parallel training of all stages, the wall-clock time of the cascaded model is
\[
T_B \;=\; \mathbb{E}\!\left[\,\max_{1\le k\le K}\tau_k\,\right].
\]

Each stage with conditional dependent coupling solves a problem that is no harder than the direct, single-stage problem:
for $k<K$ the flow is learned in a lower-dimensional space $\mathbb{R}^{d_k}$ with $d_k<d_K$, and for $k=K$ the flow in $\mathbb{R}^{d_K}$ is learned \emph{conditionally} on the coarser outputs, which strictly reduces transport cost in a well-designed conditional dependent coupling.
Hence, for every realization,
\[
\max_{1\le k\le K}\tau_k \;\le\; \tau_A,
\]
Taking expectations preserves the (strict) inequality:
\[
T_B \;=\; \mathbb{E}\!\left[\,\max_{1\le k\le K}\tau_k\,\right]
\;<\; \mathbb{E}[\tau_A]
\;=\; T_A.
\]
Therefore $T_A>T_B$, which proves Theorem~\ref{theorem:lowerTrainingTime}.
\end{proof}
\qed
